# Supplementary material for: FlexiFilm: Long Video Generation with Flexible Conditions
Source: arXiv:2404.18620 source file (2024-04-29)
Supplement: Supplementary file 1 [file supp.tex]

For training process, we first randomly sample $N$ continuous frames from each video, and then select an integer $i$ between 1 and $N$ as the conditional video frame length. Then, these $N$ frames of video perform as the target and are added noises by the scheduler, the first $i$ frames are sent to the video projector as the condition, and the number $i$ is also sent to the model as the distance condition. 

\begin{figure*}[t!]
  \centering
  \includegraphics[width=\textwidth]{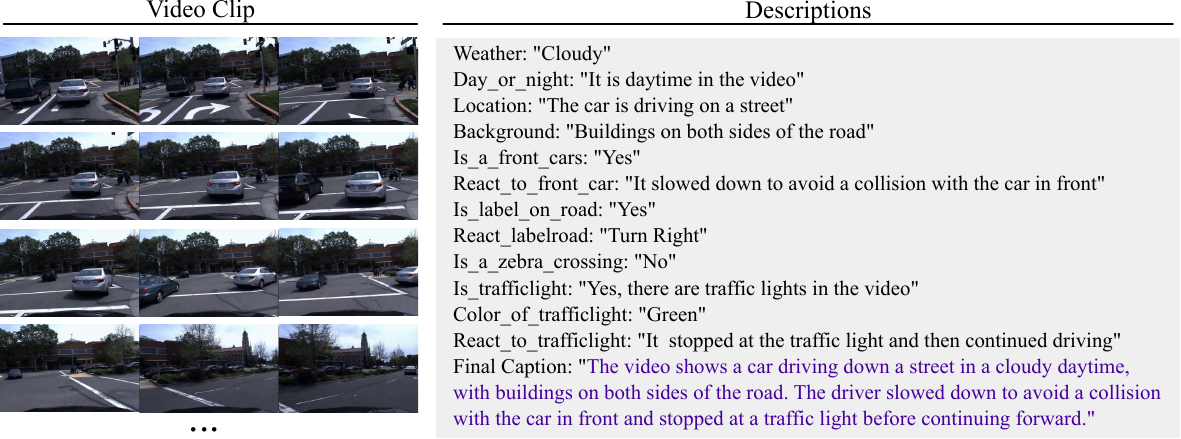}
  \caption{FF-Drive1 Dataset. Our dataset contains paired descriptions of various aspects of the video. In addition to static information such as weather, background, traffic lights, etc., it also contains dynamic information descriptions of the vehicle (for example, "it stopped at the traffic light and then continued driving"), and a long captions is summarized for each video.}
  \label{fig:dataset}
\end{figure*}
For example, for a short video generative model, the conditions may be: a image prefix and a short word or text description. While for a long video generative model, the conditions may be a short video prefix and an extremely complex text description. 
(i.e. "A car driving down a street in a cloudy daytime, with buildings on both sides of the road. The driver slowed down to avoid a collision with the car in front and stopped at a traffic light before continuing forward")

During the construction of the FF-Drive1 dataset, we carefully filtered the following content: 1. videos shorter than 20s, 2. videos of the driver’s face (Considering social ethics and privacy issues), 3. videos generated by the simulator, 4. flicker clips and color-distorted frames, 5. videos with too fast acceleration ratio. 6. videos with very small changes in optical flow (because they may be static repeating scenes). 

This dataset includes a variety of complex driving scenarios, including different weather conditions, day and night scenes, city and suburbs, as well as pedestrians crossing the road and signals changing, and an example is shown in \ref{fig:dataset}

(as shown in \ref{fig:train}, Q Template)

For the comparison of long video generation, we take into account the GPU memory limitations, and choose the settings of 80 frames and 24fps for one-go generation to compare with the baseline VideoCrafter-1. As shown in \ref{fig:exp}(3), our generation results are consistency in temporal structure during long video generation, where the time series advances steadily (i.e. the car continues to move forward, gradually surpassing the front motorcycle). In contrast, although the baseline VideoCrafter-1 is spatially faithful to the original image, it comes out unreasonable temporal loops (i.e. the content of frames 32-48 and 64-80 are basically repeated) in long video generation.

 which is faithful to the detailed and temporal nature of the text description: the first example uses 16 frames According to the condition, FlexiFilm successfully generates a scene of a car driving out of a tunnel according to the text requirements; in the second example, using an 1-frame condition, FlexiFilm generates the subsequent video of the car passing a street sign and a white car appearing in front of it according to the text requirements.

 As shown in \ref{fig:cons}, we compared the zero-shot consistency and fidelity scores of FlexiFilm and VideoCrafter on the ZOD\cite{alibeigi2023zenseact} dataset, and the results show that FlexiFilm has significantly better consistency, and comparable fidelity to the baseline. During the comparison, we set the generation task to generating 16 frames with 1 image as the reference, and the video resolution is set to 320x192.

 For the fidelity of generated videos, we define it as the degree of semantic similarity between the generated frames and the reference image. Specifically, we quantify the fidelity score of each generated video as the Clip Score between a randomly sampled generated frame and the reference image.

 We found that FlexiFilm’s FVD metric was poor, which we believe may be due to the insufficiently rich data types in the training dataset (Contains only self-driving videos), so we plan to enrich the data categories in the dataset in subsequent work. During the test, due to insufficient time, we only sampled 3,000 videos for calculation, which is not the same as the settings of baselines (most baselines sampled more than 10,000 videos). We set the task to generate a 16-frame video conditional on a single frame image and a category label. The video resolution is 320x192, while most of the generation in the baselines is 128x128 and upsampled to a resolution of 256x256 through bilinear interpolation.
